# Supplementary material for: Can We Make Code Green? Understanding Trade-Offs in LLMs vs. Human Code Optimizations
Source: arXiv:2503.20126 source file (2025-03-26)
Supplement: Supplementary file 1 [file appendix.tex]

\section{Appendix}
\label{sec:appendix}

\input{Energy-practices-on-Matlab/Tables/Themes-frequency}
